# Supplementary material for: Signatures of two-photon pulses from a quantum two-level system
Source: arXiv:1709.01120 ancillary file (2017-09-04)
Supplement: Supplementary file 1 [file Supplementary_information.pdf]

# Supplementary information: Signatures of two-photon pulses from a quantum two-level system

**Kevin A. Fischer[1†⋆], Lukas Hanschke[2†], Jakob Wierzbowski[2], Tobias Simmet[2], Constantin Dory[1], Jonathan J. Finley[2], Jelena Vučković[1], Kai Müller[2⋆]**

## Experimental excited-state lifetime

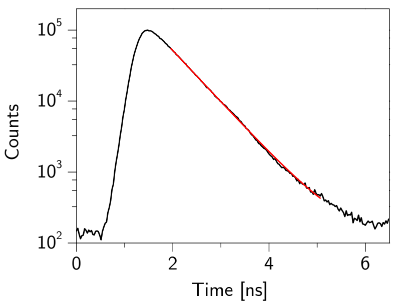


**Figure S1 | Lifetime measurement.** Time-resolved excited-state decay measurement under resonant excitation with a short (20.5 ps) pulse, data as black line. Mono-exponential fit (red) reveals a lifetime of 602 ps. This extracted lifetime is used in our quantum-optical model.

## Rabi oscillation under excitation by the 20 ps long pulse

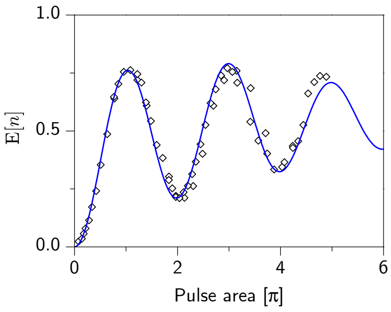


**Figure S2 | Rabi oscillation with short pulses (20.5 ps).** Measured Rabi oscillation (data points) using 20.5 ps long pulses. A fit to the data (blue line) produces excellent agreement using the same dephasing parameters obtained from fitting the Rabi oscillation for 80 ps long pulses, but with a slightly different chirp (5.4 % in bandwidth).

In the main part of the manuscript, a Rabi oscillation for 80 ps long excitation pulses was presented and fitted in order to extract the phonon-induced and noise-based dephasing rates of the quantum dot's excited state. A similar set of data is presented in Fig. S2, but for 20.5 ps long pulses. The fit produces excellent agreement with the data and, importantly, was obtained using the same dephasing parameters as extracted from the 80 ps long pulses. Moreover, using these parameters in simulation results in a value of $g^2[0] = 0.80$, which is in good agreement with the measured value discussed in the main part of the manuscript.

## Photon number variance

In Fig. 1c of the main part of the manuscript, the purity of single-photon emission and two-photon emission as a function of the pulse area were discussed for a pulse length of $\tau_{\mathrm{FWHM}} = 0.1/\Gamma$. The same data is replotted in Fig. S3 which shows the single-photon purity in green and the two-photon purity in red. In addition, the figure shows the photon number variance relative to a coherent state as a solid blue line. The variance exhibits minima for pulse areas of odd multiples of $\pi$ and maxima for even multiples of $\pi$. This quantitatively corroborates the often made assumption that exciting with a pulse area of $\pi$ is optimal for single-photon generation. For larger pulse areas the variance increases due to the addition of the two-photon state component, while for smaller pulse areas the variance increases due to the addition of the vacuum state component.

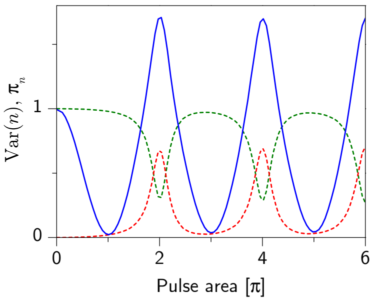


**Figure S3 | Simulated photon number variance for short pulses.** Quantum two-level system excited by short pulses of length $\tau_{\mathrm{FWHM}} = 0.1/\Gamma$. Single-photon purity $\pi_1$ (green) and two-photon purity $\pi_2$ (red) respectively exhibit minima and maxima at pulse areas of $2\pi$. The variance relative to coherent state variance is presented as a solid blue line and exhibits minima/maxima for pulse areas equal to odd/even multiples of $\pi$.

## Two-photon emission with long pulses

In the main part of the manuscript, we focused on the domain where the pulse length $\tau_{\mathrm{FWHM}}$ is relatively short compared to the lifetime of the quantum emitter $1/\Gamma$ and where the bunching is strong. However, our model also allows us to investigate the limit of arbitrarily short or long pulses. To these ends, Fig. S4a shows the purities of single (green), two (red), three

[1]E. L. Ginzton Laboratory, Stanford University, Stanford CA 94305, USA
[†]These authors contributed equally
[⋆]email: kevinf@stanford.edu; kai.mueller@wsi.tum.de
[2]Walter Schottky Institut and Physik Department, Technische Universität München, 85748 Garching, Germany

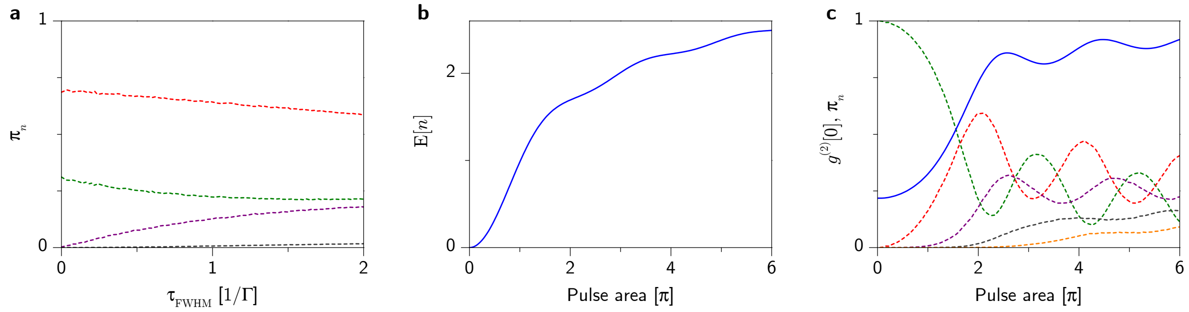


**Figure S4 | Two-photon emission with long pulses. a,** Photon number purities as a function of the pulse length: $\pi_1$ (green), $\pi_2$ (red), $\pi_3$ (purple), and $\pi_4$ (dark grey). **b,** Power dependence of total emission for long pulses ($\tau_{\mathrm{FWHM}} = 2/\Gamma$) **c,** Power dependence of $g^2[0]$ (blue) and photon purities for same pulse length as in (**b**): $\pi_1$ (green), $\pi_2$ (red), $\pi_3$ (purple), $\pi_4$ (dark grey), and $\pi_{n>4}$ (orange).

(purple), and four (grey) photon emission as a function of the pulse length for exciting with $2\pi$ pulses.

As explained in the main text, the purities asymptotically approach a dominant two-photon purity of 70 % for arbitrarily short pulses (Fig. S4a)—in this regime even the purely ideal two-level system does not emit single-photons in the manner as traditionally predicted.

On the other hand, with increasing pulse length the purities of single- and two-photon emission decrease and the probability for higher photon numbers increases. While the purity of two-photon emission remains higher than the purity of any other photon number, the presence of higher photon numbers has strong impact on the emission. For example, when looking at the power dependence of the total emission for a pulse length of $\tau_{\mathrm{FWHM}} = 2/\Gamma$ (Fig. S4b) no Rabi oscillations are observed any more. Instead, the signal monotonically increases with only some wiggling. For this pulse length, the power dependence of $g^2[0]$ and the photon purities are presented in Fig. S4c, which shows $g^2[0]$ as a solid blue line and the single, two, three, four, and higher-order photon purities as the green, red, purple, dark grey, and orange dashed lines, respectively. In contrast to shorter pulses as discussed in the main part of the manuscript, $g^2[0]$ (solid blue line) is always anti-bunched and shows only weak peaks. Nevertheless, the two-photon purity (dashed red line) shows clear peaks when the pulse area is a multiple of $2\pi$. Thus, we additionally expect that the two-photon bunching effect is robust to a wide range of system parameters and should be easy to study in many different experimental systems.
